# Supplementary material for: Non-linear Relaxation of Interacting Bosons Coherently Driven on a Narrow Optical Transition
Source: arXiv:1806.07210 ancillary file (2018-08-09)
Supplement: Supplementary file 1 [file supmat_RabiYbBec.pdf]

# Supplementary Material for: Non-linear Relaxation of Interacting Bosons Coherently Driven on a Narrow Optical Transition

M. Bosch Aguilera (1), R. Bouganne (1), A. Dareau (2), M. Scholl (3), Q. Beaufils (4), J. Beugnon(1), and F. Gerbier(1)
(1) *Laboratoire Kastler Brossel, Collège de France, ENS-PSL Research University, Sorbonne Université, CNRS, 11 place Marcelin-Berthelot, 75005 Paris*
(2) *Vienna Center for Quantum Science and Technology, TU Wien Atominstitut, Stadionallee 2, 1020 Vienna, Austria*
(3) *FARO Scanner Production GmbH, Lingwiesenstrasse 11/2, D-70825 Korntal-Münchingen and*
(4) *Laboratoire PhLAM, Bt. P5 - USTL, F-59655 Villeneuve d'Ascq*
(Dated: June 14, 2018)

### Derivation of the lossy Gross-Pitaevskii equations from a Master equation

The evolution of the system with inelastic two-body losses can be described by means of a Lindblad master equation [1] for the density matrix $\hat{\rho}$:

$$\frac{\mathrm{d}\hat{\rho}}{\mathrm{d}t} = \frac{1}{\mathrm{i}\hbar}[\hat{H},\hat{\rho}] + \mathcal{L}[\hat{\rho}], \tag{S1}$$

$$\mathcal{L}[\hat{\rho}] = \frac{\beta_{ee}}{2}\int \left[\hat{C}(\boldsymbol{r})\hat{\rho}\,\hat{C}^{+}(\boldsymbol{r}) - \frac{1}{2}\hat{C}^{+}(\boldsymbol{r})\hat{C}(\boldsymbol{r})\hat{\rho} - \frac{1}{2}\hat{\rho}\,\hat{C}^{+}(\boldsymbol{r})\hat{C}(\boldsymbol{r})\right] \mathrm{d}^3r. \tag{S2}$$

Here, we consider two-body inelastic losses in the excited state, corresponding to a dissipation operator of the form $\hat{C}(\boldsymbol{r}) = \hat{\Psi}_e^2(\boldsymbol{r})$, where $\hat{\Psi}_e(\boldsymbol{r})$ is the field operator that destroys a particle in $\boldsymbol{r}$. To obtain the Gross-Pitaevskii (GP) equations including the loss term, we calculate the evolution of the expectation value of the field operator $\langle\hat{\Psi}_e(\boldsymbol{r})\rangle \simeq \Phi_e(\boldsymbol{r},t)$:

$$\frac{\partial\langle\hat{\Psi}_e(\boldsymbol{r})\rangle(t)}{\partial t} = \frac{1}{\mathrm{i}\hbar}\mathrm{tr}\left(\hat{\Psi}_e(\boldsymbol{r})[\hat{H},\hat{\rho}]\right) + \mathrm{tr}\left(\hat{\Psi}_e(\boldsymbol{r})\mathcal{L}[\hat{\rho}]\right), \tag{S3}$$

where $\mathrm{tr}(\cdot)$ denotes the trace. The first term in the rhs of eq.(S3), equal to $-\mathrm{i}\langle[\hat{\Psi}_e(\boldsymbol{r}),\hat{H}]\rangle/\hbar$, leads to the usual GP equations [2]:

$$\mathrm{i}\hbar\frac{\partial\Phi_e(\boldsymbol{r},t)}{\partial t}\bigg|_{\hat{H}} = \left[-\frac{\hbar^2}{2m}\nabla^2 + V_{\mathrm{tr}}(\boldsymbol{r}) - \hbar\delta_{\mathrm{L}} + g_{ge}|\Phi_g(\boldsymbol{r},t)|^2 + g_{ee}|\Phi_e(\boldsymbol{r},t)|^2\right]\Phi_e(\boldsymbol{r},t) + \frac{\hbar\Omega_{\mathrm{L}}}{2}\,\mathrm{e}^{\mathrm{i}\boldsymbol{k}_{\mathrm{L}}\cdot\boldsymbol{r}}\Phi_g(\boldsymbol{r},t). \tag{S4}$$

For the second term in the rhs of eq.(S3), by using the invariance of the trace under cyclic permutations and $[\hat{\Psi}_e(\boldsymbol{r}),\hat{\Psi}_e^{+}(\boldsymbol{r}')] = \delta(\boldsymbol{r}-\boldsymbol{r}')$ we can write:

$$\frac{\partial\langle\hat{\Psi}_e(\boldsymbol{r})\rangle(t)}{\partial t}\bigg|_{\mathcal{L}} = -\frac{\beta_{ee}}{2}\langle\hat{\Psi}_e^{+}(\boldsymbol{r})\hat{\Psi}_e(\boldsymbol{r})^2\rangle. \tag{S5}$$

In the mean field approximation: $\langle\hat{\Psi}_e^{+}(\boldsymbol{r})\hat{\Psi}_e(\boldsymbol{r})^2\rangle \simeq |\Phi_e(\boldsymbol{r},t)|^2\Phi_e(\boldsymbol{r},t)$, we can absorb the contribution of the losses in the GP equations by rewriting $g_{ee}$ in the form:

$$g_{ee} \to g'_{ee} = \frac{4\pi\hbar^2}{m}a_{ee} - \mathrm{i}\frac{\hbar}{2}\beta_{ee}. \tag{S6}$$

The $\beta_{ee}$ coefficient corresponds to the parameter used in the inelastic loss-rate equation $\partial\langle\hat{\Psi}_e^{+}\hat{\Psi}_e\rangle/\partial t = -\beta_{ee}\langle\hat{\Psi}_e^{+}\hat{\Psi}_e^{+}\hat{\Psi}_e\hat{\Psi}_e\rangle$. For a BEC, this equation reduces to $\dot{\rho}_e = -\beta_{ee}\rho_e^2$ with $\rho_e = \langle\hat{\Psi}_e^{+}\hat{\Psi}_e\rangle$ the mean density in $e$ [3, 4].

## Frequency Domain Spectroscopy

In this Section, we discuss frequency domain spectroscopy of a BEC on the clock transition. We consider an atomic BEC prepared in the electronic ground state in various conditions, apply a pulse of length $t$ to transfer part of the atoms to the excited state, and record the number of remaining ground state atoms. Differently from the time-domain experiments presented in the main text, we vary the laser detuning for a fixed pulse length. We show an example of the recorded spectra in Fig.S1. The prediction of the two-component GP model from eqs.(4-5) in the main text is also shown in the same figure, in excellent agreement with the experimental curve. In the following we discuss the main physical effects (included in the GP model) determining the shape and width of the spectra, namely inhomogeneous, state-dependent interactions and Doppler broadening. Fourier broadening due to the finite pulse length can be neglected in all cases considered here. Moreover, the non-uniformity of the Rabi frequency $\Omega_{\mathrm{L}}$ over the cloud due to the finite size of the probe beam (inducing a position-dependent differential light-shift, and therefore, an inhomogeneous detuning) plays no noticeable role for the time pulses employed. We do not observe any broadening or dephasing caused by this effect in the GP simulation.

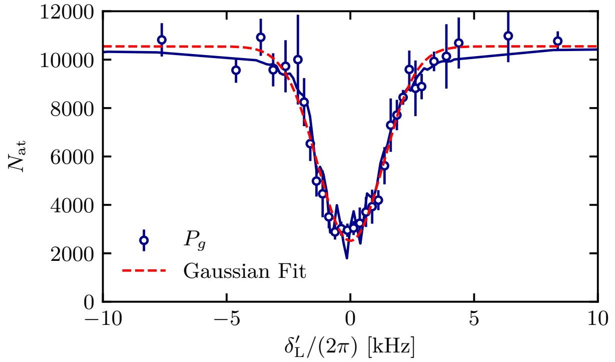


FIG. S1: Spectrum of a BEC trapped in an optical dipole trap at the magic wavelength $\lambda_{\mathrm{m}} = 759.4\,\mathrm{nm}$. Recorded atom number after time of flight $N_{\mathrm{at}}$ versus the detuning. The experimental parameters are: $\Omega_{\mathrm{L}} = 2\pi \times 150\,\mathrm{Hz}$, $t = 30\,\mathrm{ms}$ and $(\omega_x, \omega_y, \omega_z) = 2\pi \times (21, 665, 665)$ Hz. Blue dots are the experimental data points. The solid blue line is the GP simulation. The red dashed line is a Gaussian fit to the data of rms width $\sigma_{\mathrm{exp}} = 2\pi \times 1.3\,\mathrm{kHz}$.

## Theoretical description of the spectra

The spectrum of an interacting BEC in a magic dipole trap (such that the trap potential is identical for $g$ and $e$) is determined by two factors, the inhomogeneous mean-field interactions and the finite momentum width of the initial BEC leading to Doppler broadening. We consider weak excitations so that the population in the excited state can be neglected at all times. Similar situations have been discussed in the context of optical spectroscopy of hydrogen [5] and Bragg spectroscopy of ground state alkali atoms [6, 7].

One can understand qualitatively the main features of the spectra from a semi-classical argument, where each atom is taken to have a defined momentum and position. The classical energy for an atom in the ground state with momentum $\boldsymbol{p}_i$ at position $\boldsymbol{r}$ is $E_{\mathrm{i}} = E_g + \boldsymbol{p}_{\mathrm{i}}^2/(2M) + V_{\mathrm{tr}}(\boldsymbol{r}) + g_{gg}n_g(\boldsymbol{r})$, with $E_g$ the internal energy of the atom, $V_{\mathrm{tr}}(\boldsymbol{r})$ the trap potential, and the interactions have been considered in the mean-field approximation. Absorption of a photon from the probe laser promotes the atom to the excited state, changing the atomic momentum to $\boldsymbol{p}_{\mathrm{f}} = \boldsymbol{p}_{\mathrm{i}} + \hbar\boldsymbol{k}_{\mathrm{L}}$ and the energy to $E_{\mathrm{f}} = E_e + \boldsymbol{p}_{\mathrm{f}}^2/(2M) + V_{\mathrm{tr}}(\boldsymbol{r}) + g_{ge}n_g(\boldsymbol{r})$. The resonance condition (conservation of energy) is then

$$\hbar\omega_{\mathrm{L}} = E_{\mathrm{f}} - E_{\mathrm{i}} = \hbar\omega'_0 + \hbar\boldsymbol{v}_{\mathrm{R}} \cdot \boldsymbol{p}_{\mathrm{i}} + (g_{ge} - g_{gg})\, n_g(\boldsymbol{r}). \tag{S7}$$

The first term in the rhs is the bare resonance frequency $\omega_0$ corrected by the recoil frequency $\omega_{\mathrm{R}} = \hbar\boldsymbol{k}_{\mathrm{L}}^2/(2M)$, with $\omega'_0 = \omega_0 + \omega_{\mathrm{R}}$. The second term indicates that the line is Doppler-sensitive, i.e. the resonance is shifted by a quantity proportional to the momentum with respect to an atom at rest. The third term corresponds to spatially inhomogeneous broadening due to mean-field interactions.

*Doppler broadening*

Because of the confinement to a finite size $R_i$, the trapped BEC acquires a momentum width $\Delta p_i \sim \hbar/R_i$, with $R_i$ the Thomas-Fermi radius in direction $i = x, y, z$. Without interaction shift (i.e. if $g_{ge} = g_{gg}$), this leads to an inhomogeneous, Doppler- broadened resonance profile [6, 7]:

$$A_{\mathrm{D}}(\boldsymbol{q}, \delta'_{\mathrm{L}}) = \int n(\boldsymbol{p})\delta\left(\hbar\delta'_{\mathrm{L}} - \frac{\boldsymbol{p}\cdot\boldsymbol{q}}{M}\right) \mathrm{d}^3 p, \tag{S8}$$

with $\delta'_{\mathrm{L}} = \delta_{\mathrm{L}} - \omega_{\mathrm{R}}$ and $n(\boldsymbol{p})$ the momentum distribution of the initial condensate. In our case, where $\boldsymbol{q} = \hbar k_L(\cos\theta, \sin\theta, 0)$ and $R_x \gg R_y$, we have $\boldsymbol{p}\cdot\boldsymbol{q} \sim \hbar k_{\mathrm{L}} q \sin\theta$ and

$$A_{\mathrm{D}}(\boldsymbol{q}, \delta'_{\mathrm{L}}) \simeq \frac{M}{\hbar k_{\mathrm{L}} \sin\theta} \int n\left(p_x, \frac{M\delta'_{\mathrm{L}}}{k_{\mathrm{L}}\sin\theta}, p_z\right) \mathrm{d}p_x\, \mathrm{d}p_z. \tag{S9}$$

The function $A_{\mathrm{D}}$ is peaked around $\delta'_{\mathrm{L}} = 0$ provided $h/R_i \ll \hbar\omega_{\mathrm{R}}$, a condition typically well-fulfilled for BECs. By carrying out a Gaussian expansion around $\delta'_{\mathrm{L}} = 0$, the rms frequency width of this Gaussian is [7]:

$$\Delta_{\mathrm{D}} = \sqrt{\frac{8}{3}}\frac{v_{\mathrm{R}}\sin\theta}{R_y} \simeq 1.63\frac{v_{\mathrm{R}}\sin\theta}{R_y}. \tag{S10}$$

*Mean-field broadening*

If we neglect the Doppler effect, we can treat the system under the local density approximation, where the response of a small region centered at a point $\boldsymbol{r}$ is then taken to be the same as a uniform system of density $n(\boldsymbol{r})$. The total response is then obtained by integrating over $\boldsymbol{r}$. The calculation proceeds as done in [5–7]. If we define $\chi = (g_{ge} - g_{gg})/g_{gg}$, the spectrum is proportional to:

$$A_{\mathrm{int}}(\delta'_{\mathrm{L}}) \propto \frac{\hbar\delta'_{\mathrm{L}}}{\chi\mu}\sqrt{1 - \frac{\hbar\delta'_{\mathrm{L}}}{\chi\mu}}. \tag{S11}$$

We can calculate the root-mean-square (rms) frequency width of the previous expression to estimate the spectral broadening due to interactions,

$$\Delta_{\mathrm{int}} = \frac{1}{\hbar}\sqrt{\frac{8}{147}}\chi\mu \simeq 0.23\frac{\chi\mu}{\hbar}. \tag{S12}$$

**Effect of both contributions**

To take both effects into account, we model the experimental spectra by a Gaussian of rms width $\sigma$. In analogy with work on Bragg spectroscopy [6, 7], we take $\sigma$ to be given by:

$$\sigma = \sqrt{\Delta_{\mathrm{D}}^2 + \Delta_{\mathrm{int}}^2}. \tag{S13}$$

Our typical experimental values are $\mu/h \sim 1-\ 2.5\,\mathrm{kHz}$, $R_y \sim 0.7-1.4\,\mu\mathrm{m}$, and $\theta = \pi/4$. Moreover, in our case $g_{ge} = 0.9\, g_{gg}$ ($\chi = 0.1$), so that $\Delta_{\mathrm{int}}/(2\pi) \sim 25-60\,\mathrm{Hz}$ is small compared to the Doppler contribution $\Delta_{\mathrm{D}}/(2\pi) \sim 500-1000\,\mathrm{Hz}$.

A similar heuristic Gaussian model has been used previously to describe Bragg spectroscopy experiments [6, 7]. We have compared the heuristic model with the Gross-Pitaevskii model described in the main text [eqs. (4,5)]. To make this comparison, we computed spectra in conditions similar to the ones used in the experiments, only modifying the trap confinement and probe pulse length to ensure, i) that the probing pulse is shorter than a quarter of the trap period (so that the motion of the atoms is essentially the same as in free space), and ii) that the depletion is weak enough (so that we are in the perturbative regime where the analytical results are valid). The results are shown in Fig.S2, and we find a good agreement between the GP simulation and the heuristic model in eq. (S13).

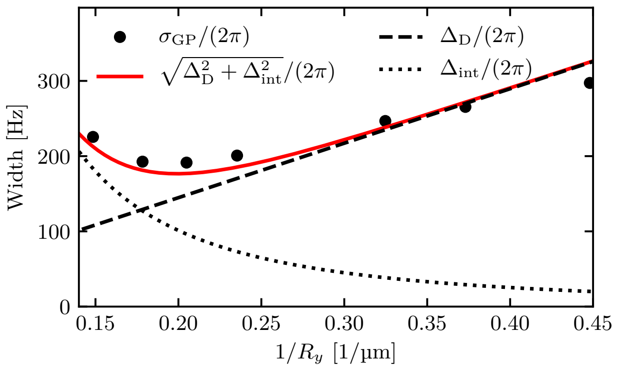


FIG. S2: Spectrum width as a function of the inverse of the Thomas-Fermi radius $R_y$ in the $y-$direction. Black dashed and dotted lines correspond to the interaction and Doppler widths, respectively. The red solid line is the quadrature sum of both contributions. The points correspond to the rms of a Gaussian fit to spectra simulated via the GP equations. The parameters for the simulation are: $\Omega_L = 2\pi \times 25\,\text{Hz}$ , $t = 3.5\,\text{ms}$, $(\omega_x, \omega_y, \omega_z) = 2\pi \times (10, 100, 100)$ Hz and $\chi$ is set to $\chi = 0.2$. The Thomas-Fermi radius is varied by changing the atom number from $N = 2 \times 10^4$ atoms to $N = 5 \times 10^6$ atoms.

### Comparison with experiments

We analyze experimental spectra as in Fig.S1 by performing a Gaussian fit and extracting the rms width $\sigma_{exp}$ from these fits. We also generated theoretical spectra under the same conditions as in the experiments by using the GP eqs.$(4-5)$ of the main text and using the same procedure to extract an rms width $\sigma_{GP}$. Both widths and the predictions from the heuristic model eq. (S13) are shown in Fig.S4. We find that $\sigma_{exp}$ and $\sigma_{GP}$ roughly agree, although the former is slightly larger. This could be due to additional experimental fluctuations, for instance of the probe laser frequency or power, or of the atom number.

Both $\sigma_{exp}$ and $\sigma_{GP}$ are above the heuristic width $\sigma$ from eq. (S13). The mismatch can be ascribed to the fact that we used long pulse times with substantial depletion in the experiments (and in the GP calculations). In these conditions, the assumption of a perturbative transfer leading to eq. (S13) is no longer satisfied.

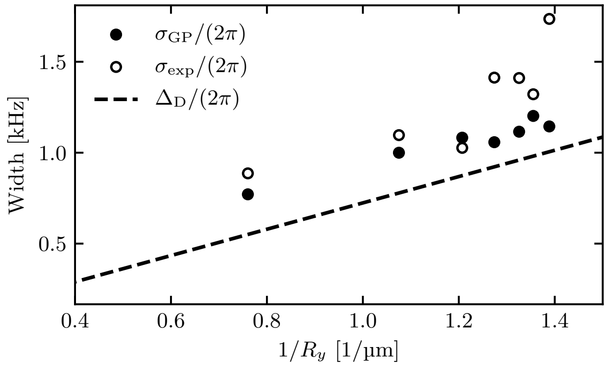


FIG. S3: Spectrum width as a function of the inverse of the Thomas-Fermi radius $R_y$ in the $y-$direction. The black dashed line corresponds to the width predicted by eq.(S10). Empty points correspond to the rms width of a Gaussian fitted to the experimental data (see Fig.S1). Filled points correspond to the rms of a Gaussian fit to spectra simulated via the GP equations. The experimental parameters are $\Omega_L = 2\pi \times 150\,\text{Hz}$ and the pulse length $t = 20 - 30\,\text{ms}$. The Thomas-Fermi radius is varied by using different trapping frequencies and the atom number.

### Determination of the resonance frequency in Rabi oscillations experiments

Before acquiring a time-resolved curve as in Figs.(1b-f, 4a) in the main text, we record a spectrum to determine the resonance center frequency in order to correct for possible cavity drifts. We set the laser detuning for each time-resolved curve at the center of the spectrum, determined by a Gaussian fit as in Fig.S1. We now try to estimate the error induced by this procedure in pointing the center frequency (and therefore on the subsequent detuning $\delta'_{\rm L} = \delta_{\rm L} - \omega_{\rm R}$ of the laser during a time-resolved experiment). We record spectra with a sampling $\delta f_{\rm sampling}/(2\pi) = 500\,{\rm Hz}$, with one repetition per sampling value. We estimate the error made in pointing the center of the spectra by evaluating the standard deviation of the mean, $\delta\omega_{\rm L} \leq a\sigma_{\rm exp}/\sqrt{N_*}$, with $\sigma_{\rm exp}/(2\pi) \simeq 3\,{\rm kHz}$ the rms width of the measured spectra and $N_* = \sigma_{\rm exp}/\delta f_{\rm sampling}$ the number of data points with significant statistical weight and $a$ a numerical factor. The order of magnitude of the pointing error is then a fraction of $\sqrt{\delta f_{\rm sampling}\sigma_{\rm exp}} \simeq 2\pi \times 1\,{\rm kHz}$. This is consistent with the fits of the Rabi oscillations performed by using the two-component GP model, where we let the detuning $\delta'_{\rm L}$ free. We find for all experiments $|\delta'_{\rm L}| \leq 2\pi \times 300\,{\rm Hz}$, which is within the uncertainty range estimated above.

### Numerical Algorithm

To perform the fits, we use a dimensionless form of eqs.$(4-5)$ in the main text using harmonic oscillator units corresponding to the smallest frequency $\omega_x$. We work with a cartesian $40 \times 40 \times 40$ grid. The size of the grid in each direction corresponds to $4R_i$ with $R_i$ $(i = x, y, z)$ the Thomas-Fermi radius of the condensate. We choose the time step as $\Delta {\tt t}_k = 1/(100\omega_y)$, with $\omega_y$ the highest trapping frequency $(\omega_x \Delta {\tt t}_k \simeq 2 \times 10^{-4})$. We solve the GP equations using the split-step Fourier method where the kinetic energy and local terms are propagated separately and locally in momentum and position spaces, respectively. The term coupling $g$ and $e$ is implemented exactly by performing explicitly a $SU(2)$ rotation with parameters determined by the local position-dependent detuning and the Rabi frequency.

### Empirical Fit

In this section, we show for completeness some of the fits performed by using eq.(3) in the main text.

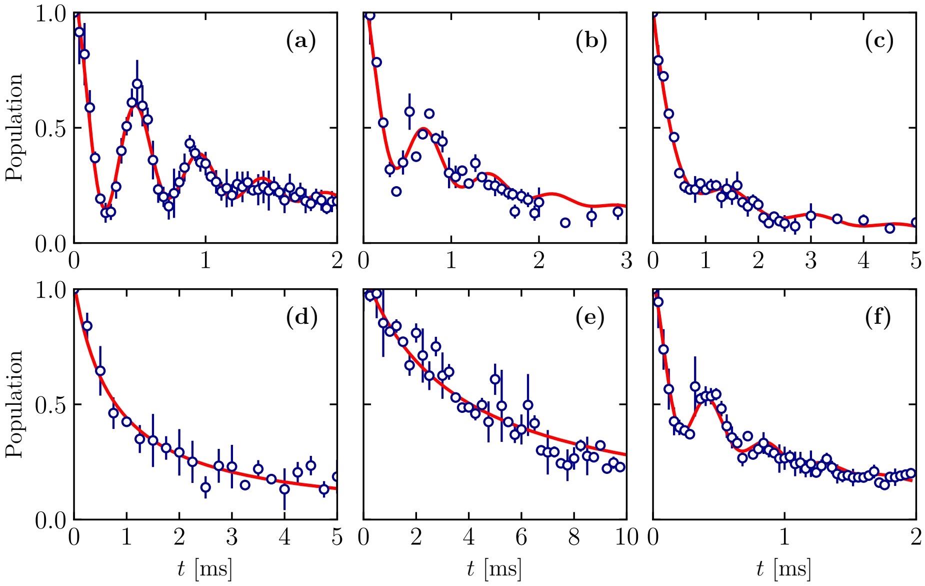


FIG. S4: Population dynamics as a function of pulse duration $t$ for different Rabi frequencies: **(a):** $\Omega_{\rm L}/(2\pi) = 2.1\,{\rm kHz}$, **(b):** $\Omega_{\rm L}/(2\pi) = 1.1\,{\rm kHz}$, **(c):** $\Omega_{\rm L}/(2\pi) = 750\,{\rm Hz}$, **(d):** $\Omega_{\rm L}/(2\pi) = 540\,{\rm Hz}$, **(e):** $\Omega_{\rm L}/(2\pi) = 200\,{\rm Hz}$ and **(f):** $\Omega_{\rm L}/(2\pi) = 2\,{\rm kHz}$. The chemical potential for **(a)**-**(e)** is $\mu/h \simeq 1\,{\rm kHz}$, and for **(f)** is $\mu/h \simeq 2\,{\rm kHz}$. The red solid line corresponds to a fit performed using eq.(3) in the main text. Figures **(a)**-**(e)** correspond to Fig.1(b-f) in the main text and figure **(f)** corresponds to Fig.4**a** in the main text.

[1] S. Haroche and J. Raimond, *Exploring the Quantum* (Oxford University Press, Oxford, 2006).
[2] L. Pitaevskii and S. Stringari, *Bose-Einstein condensation* (Oxford University Press, Oxford, 2003).
[3] Y. Kagan, B. Svistunov, and G. Shlyapnikov, Soviet Journal of Experimental and Theoretical Physics Letters **42**, 209 (1985).
[4] W. Ketterle and H.-J. Miesner, Phys. Rev. A **56**, 3291 (1997).
[5] T. C. Killian, Phys. Rev. A **61**, 033611 (2000).
[6] J. Stenger, S. Inouye, A. P. Chikkatur, D. M. Stamper-Kurn, D. E. Pritchard, and W. Ketterle, Phys. Rev. Lett. **82**, 4569 (1999).
[7] F. Zambelli, L. Pitaevskii, D. M. Stamper-Kurn, and S. Stringari, Phys. Rev. A **61**, 063608 (2000).
